# Supplementary material for: Spatiotemporal Flux Probing for Single-Photon Videography
Source: arXiv:2609.22479 source file (2026-09-18)
Supplement: Supplementary file 2 [file supp_notation.tex]

\definecolor{lightgray}{gray}{0.8}
\definecolor{lightgreen}{rgb}{0.74,0.96,0.65}
\definecolor{commentgreen}{rgb}{0,0.4,0.26}
\definecolor{commentblue}{rgb}{0.1,0.1,0.6}
\definecolor{lightred}{rgb}{0.96,0.74,0.65}
\definecolor{cvprblue}{rgb}{0.21,0.49,0.74}

\newcommand{\changeS}[1]{\textcolor{commentgreen}{\em {\bf Sotiris:} #1}}
\newcommand{\changeJ}[1]{\textcolor{commentblue}{\em {\bf Jerry:} #1}}
\newcommand{\changeM}[1]{\textcolor{lightgreen}{Matteo#1}}
\newcommand{\sid}[1]{\textcolor{blue}{{\em {\bf Sid:} #1}}}
\newcommand{\sidp}[1]{\textcolor{black}{{\em #1}}}
\newcommand{\changeA}[1]{\textcolor{purple}{\em {\bf Andrew:} #1}}
\newcommand{\revision}{\textcolor{red}}

\newcommand{\hidesectionfigures}{false}

\newcommand{\aka}{\emph{a.k.a.}\xspace}

\theoremstyle{definition}
\newtheorem{definition}{Definition}
\theoremstyle{definition}
\newtheorem{proposition}{Proposition}
\theoremstyle{definition}
\newtheorem{lemma}{Lemma}
\theoremstyle{definition}
\newtheorem{corollary}{Corollary}
\theoremstyle{definition}
\newtheorem{paperequation}{Equation}
\newtheorem*{remark}{Remark}

\newcommand{\eqcomma}{\ \ ,}
\newcommand{\eqstop}{\ \ .}
\renewcommand{\eqref}[1]{Eq.~\ref{#1}}

\newcommand{\vecind}[2]{{#1}({#2})}
\newcommand{\ind}[2]{{#1}_{#2}}
\newcommand{\setind}[2]{{#1}_{#2}}
\newcommand{\funcind}[2]{{#1}({#2})}
\newcommand{\upind}[2]{{#1}^{#2}}
\newcommand{\norm}[2]{\|{#1}\|_{#2}}
\newcommand{\floor}[2]{#2\lfloor #1 #2\rfloor}

\newcommand{\albedo}{\alpha}
\newcommand{\illumination}{A}
\newcommand{\background}{B}
\newcommand{\lightspeed}{c}
\newcommand{\lossparamsb}{c}
\newcommand{\depth}{{d}} %
\newcommand{\error}{e}
\newcommand{\freq}{f}
\newcommand{\angfreq}{\omega}
\newcommand{\freqcand}{\mathcal{F}_\text{cand}}
\newcommand{\freqrefine}{\mathcal{F}_\text{loc}}
\newcommand{\freqdom}{\mathcal{F}_\text{rep}}
\newcommand{\probe}{p}
\newcommand{\timestampind}{i}
\newcommand{\im}{j}
\newcommand{\fourierfreq}{k}
\newcommand{\light}{l} %
\newcommand{\lightind}{\light}
\newcommand{\loss}{l}
\newcommand{\brdf}{L}
\newcommand{\lightset}{\mathcal L}
\newcommand{\lossfunc}{\mathcal L}
\newcommand{\pathlength}{m}
\newcommand{\counting}{n}
\newcommand{\harmonic}{n}
\newcommand{\neighborhood}{\mathcal N}
\newcommand{\normaldist}{{\mathcal N}}
\newcommand{\numneigh}{\num{n}}
\newcommand{\sync}{o}
\newcommand{\cfarprob}{p}
\newcommand{\pixind}{q}
\newcommand{\pix}{q}
\newcommand{\pixset}{\mathcal{Q}}
\newcommand{\reflectsym}{r}
\newcommand{\scene}{s}
\newcommand{\sphere}{S}
\newcommand{\timesym}{t} 
\newcommand{\period}{T}
\newcommand{\timestamps}{\mathcal{T}}
\newcommand{\timeIntSym}{u}
\newcommand{\ray}{v} %
\newcommand{\visible}{v}
\newcommand{\timestamp}{\tau}
\newcommand{\real}{\mathbb{R}}

\newcommand{\amplitude}{\alpha}
\newcommand{\lossparamsa}{\alpha}
\newcommand{\sbrsym}{\beta}
\newcommand{\impulse}{\delta}
\newcommand{\cfarthresh}{\Delta}
\newcommand{\direction}{\theta}
\newcommand{\flux}{\phi}
\newcommand{\stpflux}{\phi (x,y,t)}
\newcommand{\fftflux}{\Phi}
\newcommand{\pulse}{\psi}
\newcommand{\fftpulse}{{\Psi}}
\newcommand{\phase}{\phi}
\newcommand{\robustloss}{\rho}
\newcommand{\radiance}{\Phi}
\newcommand{\tof}{\tau}
\newcommand{\spacevol}{v}

\newcommand{\ambient}{\text{ambient}}
\newcommand{\DC}{\text{DC}}
\newcommand{\R}{\mathbb{R}}
\DeclareMathOperator{\FT}{\mathcal{F}}

\newcommand{\exposure}{\timesym_{\text{exp}}}

\newcommand{\impulsetrain}[1]{\Sha_{#1}}

\newcommand{\spheresym}[1]{\setind{\sphere}{#1}}

\newcommand{\lightloc}[1]{\expandafter\ifx\expandafter\relax
\detokenize{#1}\relax\mathbf{\light}\else {\mathbf{\light}}_{#1}\fi}
  
\newcommand{\radiancefunc}[1]{\ind{\radiance}{#1}}
\newcommand{\lightdir}[1]{\ind{\direction}{#1}}
\newcommand{\illumfunc}[1]{\ind{\illumination}{#1}}
\newcommand{\syncsym}[1]{\upind{\sync}{#1}}
\newcommand{\tofsym}[1]{\expandafter\ifx\expandafter\relax
  \detokenize{#1}\relax\tof\else \upind{\tof}{#1}\fi}
\newcommand{\freqsym}[1]{\ind{\freq}{#1}}
\newcommand{\pathlengthsym}[1]{\upind{\pathlength}{#1}}
\newcommand{\periodsym}[1]{\upind{\period}{#1}}
\newcommand{\ambientsym}[1]{\ind{\ambient}{#1}}

\newcommand{\viewray}[1]{\mathbf{\ray}({#1})}

\newcommand{\viewdir}[1]{\ind{\direction}{#1}}
\newcommand{\timestampsym}[1]{\ind{\timestamp}{#1}}
\newcommand{\brdfsym}[1]{\ind{\brdf}{#1}}
\newcommand{\albedosym}[1]{\expandafter\ifx\expandafter\relax
  \detokenize{#1}\relax\albedo\else \vecind{\albedo}{#1}\fi}

\newcommand{\depthsym}[1]{\depth({#1})}

\newcommand{\sceneloc}[1]{\vecind{\mathbf{\scene}}{#1}}
\newcommand{\pixsym}[1]{\ind{\pix}{#1}}

\newcommand{\pixvec}{\mathbf{\pixind}}

\newcommand{\fluxfunc}[1]{\flux{(#1)}}
\newcommand{\fluxfuncs}[2]{\flux_{#1}({#2})}
\newcommand{\fluxfunct}[2]{\fluxfunc{{#1},{#2}}}
\newcommand{\fluxfuncst}[3]{\fluxfuncs{#1}{{#2},{#3}}}

\newcommand{\estfluxfunct}[2]{\widehat{\flux}({#1},{#2})}
\newcommand{\estfluxfuncts}[3]{\widehat{\flux}_{#1}({#2},{#3})}

\newcommand{\fftfluxp}[1]{\fftflux({#1})}
\newcommand{\fftfluxs}[1]{\fftflux_{#1}}
\newcommand{\fftfluxsp}[2]{\fftfluxs{#1}({#2})}
\newcommand{\fftfluxpf}[2]{\fftfluxp{{#1},{#2}}}
\newcommand{\fftfluxspf}[3]{\fftfluxsp{#1}{{#2},{#3}}}

\newcommand{\estfftfluxpf}[3]{\widehat{\fftflux}({#1},{#2},{#3})}
\newcommand{\estfftfluxspf}[4]{\widehat{\fftflux}_{#1}({#2},{#3},{#4})}

\newcommand{\albedofunc}[1]{\albedo{(#1)}}
\newcommand{\albedofuncs}[2]{\albedo_{#1}{(#2)}}

\newcommand{\tofs}[1]{\tof_{#1}}
\newcommand{\toffuncs}[2]{\tofs{#1}{({#2})}}

\newcommand{\freqs}[1]{\freq_{#1}}
\newcommand{\periods}[1]{\period_{#1}}
\newcommand{\syncs}[1]{\sync_{#1}}

\newcommand{\pulsefuncs}[1]{\pulse_{#1}}
\newcommand{\pulsefuncst}[2]{\pulsefuncs{#1}{({#2})}}

\newcommand{\fftpulses}[1]{\fftpulse_{#1}}
\newcommand{\fftpulsesf}[2]{\fftpulses{#1}({#2})}
\newcommand{\pulseftsf}[3]{\pulsefts{#1}{{#2},{#3}}}

\newcommand{\cfardetector}[3]{\cfarthresh({#1},{#2},{#3})}

\newcommand{\estifluxfunc}[1]{\widehat{\flux}_{#1}}

\newcommand{\fouriersym}[1]{\mathfrak{F}#1}
\newcommand{\fourier}[1]{\MakeUppercase{#1}}
\newcommand{\fluxfft}[1]{\widehat\Phi_{#1}}

\newcommand{\deltaf}[1]{\impulse{(#1)}}

\newcommand{\esti}[1]{\widehat{#1}}
\newcommand{\rv}[1]{\MakeUppercase{#1}}
\newcommand{\countingProcess}[1]{\rv{\counting}({#1})}
\newcommand{\errorsym}[1]{\ind{\error}{#1}}

\newcommand{\expectation}[1]{\mathbb{E}\bigl[\,{#1}\bigr]\;}
\newcommand{\probability}[1]{\mathbf{Pr}(#1)}
\newcommand{\variance}[1]{\mathbf{Var}[#1]}

\newcommand{\num}[1]{\MakeUppercase{#1}}
\newcommand{\numlights}{\num{\light}}
\newcommand{\numpixel}{\num{\pix}}
\newcommand{\locussym}{\Omega}
\newcommand{\numharmonics}{\num{\harmonic}}

\newcommand{\probemeas}{\mathcal{E}}
\newcommand{\probemeasnorm}{\widetilde{\probemeas}}
\newcommand{\probeFunc}[1]{p_{#1}}
\newcommand{\probeFuncGen}[1]{p(#1)}
\newcommand{\probemean}{\boldsymbol{\mathrm{\mu}}}
\newcommand{\probecov}{\boldsymbol{\mathrm{\Sigma}}}

\newcommand{\spacetime}{\mathbf{x}}
\newcommand{\spacex}{x}
\newcommand{\spacey}{y}
\newcommand{\spacexy}{\mathbf{r}}
\newcommand{\setspace}{A}
\newcommand{\setspacetime}{\Omega}
\newcommand{\setspacetimesub}{W}
\newcommand{\freqx}{\freq_{\spacex}}
\newcommand{\freqy}{\freq_{\spacey}}
\newcommand{\freqt}{\freq_{\timesym}}
\newcommand{\probespacetime}{\probe(\spacex, \spacey, \timesym)}
\newcommand{\probefreqenergy}{\probeFunc{\frecvec}^\epsilon(\events)}

\newcommand{\width}{w}
\newcommand{\height}{h}
\newcommand{\frames}{N_t}

\newcommand{\spacetimeflux}{\fluxfunc{\spacex, \spacey, \timesym}}
\newcommand{\fluxmeas}{\Phi}

\newcommand{\arrivalRate}[1]{\flux({#1})}

\newcommand{\velocity}{v}
\newcommand{\velocityVec}{\mathbf{\velocity}}

\newcommand{\intensity}[1]{i(#1)}
\newcommand{\fftintensity}[1]{I(#1)}

\newcommand{\freqvec}{\mathbf{\freq}}
\newcommand{\angfreqvec}{\boldsymbol{\angfreq}}
\newcommand{\window}{w}
\newcommand{\patch}{\mathcal{P}}
\newcommand{\freqsall}{\mathcal{F}}
\newcommand{\freqscfar}{\freqsall_{\text{det}}}

\newcommand{\event}{\mathbf{x}}
\newcommand{\events}{\mathcal{P}}
\newcommand{\eventpol}{\sigma}
\newcommand{\dvsevs}{\mathcal{V}}
\newcommand{\spikes}{\mathcal{S}}

\newcommand{\cfarsigval}{\alpha}
\newcommand{\cfarsigvalvel}{\cfarsigval_{\text{vel}}}
\newcommand{\critvalue}{c_\cfarsigval}

\newcommand{\martingale}{M}
\newcommand{\martingaleprobe}{\martingale_{\probe}}
\newcommand{\filt}{\mathbf{F}}

\newcommand{\baeventrate}{\lambda_{\text{BA}}}
