# Supplementary material for: Spatiotemporal Flux Probing for Single-Photon Videography
Source: arXiv:2609.22479 source file (2026-09-18)
Supplement: Supplementary file 3 [file supp_packages.tex]

\usepackage{etex} %

\usepackage{setspace}

\usepackage{times}
\usepackage[OT2,T1]{fontenc}
\DeclareMathAlphabet{\mathcal}{OMS}{cmsy}{m}{n}

\usepackage[ruled,vlined]{algorithm2e} %
\renewcommand{\algorithmcfname}{Pseudocode}

\usepackage{xcolor} %
\usepackage{ifpdf} %
\usepackage{ifthen} %

\usepackage{bbm}
\usepackage{soul}  
\usepackage{titlesec}

\usepackage{tikz} 
\usetikzlibrary{arrows.meta,calc,decorations.markings,math,arrows.meta}

\usepackage[percent]{overpic}
 

\usepackage{epstopdf}[update,prepend] 

\usepackage{rotate}

\usepackage{pstool}[crop=pdfcrop,cleanup={}] 

\usepackage{amsmath}
\usepackage{amsfonts}
\usepackage{amsthm}
\usepackage{amssymb}

\usepackage{diffcoeff} %

\setlength{\marginparwidth}{2cm}
\usepackage[disable]{todonotes} 

\usepackage[draft,authormarkup=none]{changes}

\usepackage{mathtools} %
\usepackage{array}       %
\usepackage{multirow}    %
\usepackage{booktabs}    %
\usepackage[noend]{algpseudocode}

\usepackage{comment}     %
\usepackage{verbatim} %

\usepackage{parskip}  %
\usepackage{placeins}
\usepackage{xspace}
\usepackage{setspace}
\usepackage{tabto}
\usepackage[export]{adjustbox}
\usepackage{diagbox}
\usepackage{makecell}
\usepackage{paralist}
\usepackage{afterpage}
\usepackage{lipsum}
\usepackage{blindtext}

\usepackage[numbers,sort&compress]{natbib} 

\usepackage[pagebackref,breaklinks=true,colorlinks=true,allcolors=cvprblue,bookmarks=false,pagebackref]{hyperref}

\usepackage{hypernat} %

\usepackage[labelfont=bf,textfont=rm,font=small]{caption} %
\captionsetup{position=bottom,font=small,labelformat=original,labelsep=colon} 
\newlength\figureheight
\newlength\figurewidth

\usepackage{amsmath}    %
\usepackage{amssymb}    %
\usepackage{amsthm}     %
\usepackage{enumitem}   %

\renewcommand{\theequation}{\thesection.\arabic{equation}}

\renewcommand{\thefigure}{\thesection.\arabic{figure}}

\SetArgSty{}
\SetKwComment{tcc}{\hspace{0pt}\#~}{}
\SetStartEndCondition{ }{}{}%
\SetKwProg{Fn}{def}{\string:}{}
\SetKwFunction{Range}{range}%
\SetKw{KwTo}{in}\SetKwFor{For}{for}{\string:}{}%
\SetKwIF{If}{ElseIf}{Else}{if}{:}{elif}{else:}{}%
\SetKwFor{While}{while}{:}{fintq}%
\newcommand{\forcond}{$i$ \KwTo\Range{$n$}} 
\AlgoDontDisplayBlockMarkers\SetAlgoNoEnd%

\titleformat{\paragraph}[runin] %
  {\normalfont\bfseries}       %
  {}                           %
  {0pt}                        %
  {}                           %

\titlespacing*{\paragraph}{0pt}{1ex}{0.25em} %
\renewcommand\paragraph[1]{\textbf{#1:}}

\usepackage[percent]{overpic} %
\usepackage{xcolor} %
\usepackage{array} %
