# Supplementary material for: Spatiotemporal Flux Probing for Single-Photon Videography
Source: arXiv:2609.22479 source file (2026-09-18)
Supplement: Supplementary file 4 [file supp_preamble.tex]

\newcommand{\red}[1]{{\color{red}#1}}
\newcommand{\TODO}[1]{\textbf{\color{red}[TODO: #1]}}
